# Supplementary material for: A framework for coupled deformation-diffusion analysis with application to degradation/healing
Source: arXiv:1106.2327 source file (2011-06-12)
Supplement: Supplementary file 1 [file S6_Appendix.tex]

%********************************************************;
%                                                        ;
%  Section: Appendix on uniform triaxial tension tests   ;
%                                                        ;
%********************************************************;
\section*{APPENDIX}
\label{Sec:Appendix}
%
%------------------------------------;
%  Remark: Diffusivity Measurements  ;
%------------------------------------;
Investigation and understanding of the material behaviour in general 
three-dimensional environments are quite demanding and time consuming. 
This is because of experimental difficulties in producing such types 
of stresses and the humongous cost involved in designing and development 
of such complex testing machines. For completeness, we just briefly 
various tri-axial experimental setups which can help experimentalists 
in determining the coefficients related to equations 
(\ref{Eqn:Coupled_diffusivity}) and (\ref{Eqn:Coupled_diffusivity_compression}) 
for various materials by appropriate modifications in order to test diffusivities 
of these materials:
Various experimental techniques for tri-axial testing have been 
proposed in the literature for different materials. 

\begin{enumerate}
\item A method for tensile testing of brittle materials such as 
  calestone (a dental plaster), copper and aluminium alloys, 
  austenitic stainless steel were described by Cridland and 
  Wood \cite{Cridland_Wood_IJFM_1968_v4_p277}, Hayhurst and 
  Felce \cite{Hayhurst_Felce_EFM_1986_v25_p645} and Calloch 
  and Marquis \cite{Calloch_Marquis_IJP_1999_v15_p521}
\item Advanced tri-axial testing of geomaterials such as rock and 
  soil were carried out by Donaghe et. al. \cite{Donaghe_Chaney_Marshall}, 
  Hunsche \cite{Cristescu_Gioda} and Wawersik 
  \cite{1997_Wawersik_Carlson_Holcomb_Williams_IJRMMS_v34_p330}.
\item Various works on generating hydrostatic tensile stresses via 
`Poker-Chip tests' on polymeric materials by Lindsey and co-workers 
\cite{1963_Lindsey_Schapery_Williams_Zak, 1966_Lindsey_PhDThesis_CIT,
  1967_Lindsey_JAP_v38_p4843}.
\end{enumerate}
